# Supplementary material for: Unsupervised Instance and Subnetwork Selection for Network Data
Source: arXiv:2212.12771 source file (2022-12-24)
Supplement: Supplementary file 1 [file 8_supp.tex]

\newpage
\clearpage
\section*{Supplementary material}
\subsection{Additional instance selection experiments}
% \todo{discuss}
We next show the experiments of instance selection and outlier detection of the Liver dataset. 
\begin{figure} [!h] 
    \footnotesize
    \centering
    \begin{subfigure}[h]{0.235\textwidth}
        \centering
        \includegraphics[width=\textwidth]{images/liver_is_3.eps}
        \caption{Feature selection} \label{fig:Liver_is_accuracy}
    \end{subfigure}
     \begin{subfigure}[h]{0.235\textwidth}
        \centering
        \includegraphics[width=\textwidth]{images/liver_outlier_roc.eps}
        \caption{Outlier detection} \label{fig:Liver_ourlier_roc}
    \end{subfigure}
    \caption{Comparison of feature selection~(\subref{fig:Liver_is_accuracy}) and outlier detection~(\subref{fig:Liver_ourlier_roc}) on the Liver dataset.}
    \label{fig:whole_is_liver}\vsa\vsb
\end{figure}

\subsection*{Additional joint feature and instance selection experiments in Liver and Embryo}
Tables~\ref{table:fs_is_evaluation_liver},\ref{table:fs_is_evaluation_embro} show the accuracy of \ourmeth for different-size subsets of features and instances in Liver and Embryo. Notably the best performance (bold for each feature set size) in both datasets is obtained without using all instances. In Liver the performance with $60\%$ and $10\%$ reaches $93.4\%$ exceeding that for all features/instances. Interestingly, 
the best performance in Embryo is obtained with as few as $20\%$ of the features and only $10\%$ of the instances resulting in $17.6\%$ accuracy gain over that of all instances/features.
In other words, small portion of representative instances contain sufficient information, demonstrating the necessity of joint feature and instance selection.
\begin{table}[!h]
\footnotesize
\begin{tabular}{|l|l|l|l|l|l|l|l|l|l|l|}
\hline
\multirow{2}{*}{\# Feature } & \multicolumn{10}{l|}{    \#  Query 
instance}           \\ \cline{2-11} 
                            & 10\% & 20\% & 30\% & 40\% & 50\% & 60\% & 70\% & 80\% & 90\% & 100\% \\ \hline
10\%                          &  75.4  &  72.1  &   82.0 &  83.6  &  85.2  & {\bf  93.4} & 90.2   &  90.2  &  90.2  &   93.4   \\ \hline
20\%                          &  75.4  &  72.1   &  83.6  &  83.6   & 86.9   &   {\bf 91.8}  &  88.5  & 91.8   & 90.2   &  91.8   \\ \hline
30\%                          &  75.4  &  73.8  & 83.6    & 85.2   & 86.9    &   {\bf 91.8}   &90.2    & 90.2   & 91.8   &   91.8    \\ \hline
40\%                          &  75.4  &  73.8  & 83.6    &  85.2  & 86.9    &    {\bf 91.8}  &90.2    & 91.8   &  90.2  &   91.8    \\ \hline
50\%                          & 75.4   &  75.4  & 83.6    & 85.2   &  86.9   &  90.2  &  90.2  &  {\bf 91.8}   & 91.8   &    91.8   \\ \hline
60\%                          &  75.4  &  73.8  & 83.6    &  83.6  & 88.5   &    {\bf 91.8} &  90.2  & 91.8   &  91.8  &    91.8   \\ \hline
70\%                          &  75.4  &  75.4   & 83.6    & 83.6   & 88.5   &    {\bf 91.8}  & 90.2   & 91.8   &  91.8  &  91.8     \\ \hline
80\%                          & 75.4   &  75.4   & 82.0   &  83.6  & 88.5   &   90.2 &  88.5  &  {\bf 91.8}   & 90.2   &    91.8   \\ \hline
90\%                          &  75.4  &   75.4  & 82.0   &  82.0  &  86.9  &   90.2  &  88.5  &  {\bf 91.8}   & 90.2   &   91.8    \\ \hline
100\%                         &  75.4  &   75.4  & 82.0   &  83.6  & 86.9   &   86.9 & 86.9  &   {\bf 90.2}  &  90.2  &    91.8   \\ \hline
\end{tabular}
\caption{\footnotesize Classification accuracy for varying number of features and instances (Liver) }
\label{table:fs_is_evaluation_liver}%\vsa\vsa
\end{table}

\begin{table}[!h]
\footnotesize
\begin{tabular}{|l|l|l|l|l|l|l|l|l|l|l|}
\hline
\multirow{2}{*}{\# Feature} & \multicolumn{10}{l|}{\#Query instance}           \\ \cline{2-11} 
                            & 10\%  & 20\%  & 30\%  & 40\%  & 50\%  & 60\%  & 70\%  & 80\%  & 90\%  & 100\%  \\ \hline
10\%       & 58.8                  &  58.8   &  {\bf 64.7}  &   58.8 &  52.9  &  58.8   &  47.0  &  58.8   &  52.9  &      52.9   \\ \hline
20\%       & {\bf 82.3}                     & 58.8    & 70.5   &  64.7  &   58.8  &  64.7  & {\bf 64.7}   &   52.9 &  58.8  &    52.9     \\ \hline
30\%      & 58.8                       & 58.8    &  {\bf 76.4}  &   58.8  &  58.8   &   58.8  &   58.8  &   58.8 &   52.9 &   52.9      \\ \hline
40\%       &   58.8                   & 58.8    &  {\bf 76.4 } & 64.7   &  58.8   &   58.8  &  64.7   &  64.7  &  64.7  &     70.5    \\ \hline
50\%       &58.8                       & 58.8    &  {\bf 76.4 }  &   58.8  &   58.8  &  64.7  &   70.5 & 64.7   &  64.7  &    64.7     \\ \hline
60\%       &58.8                       & 70.5    & 76.4   & 70.5   & 64.7   &  64.7  &  {\bf 76.4  }&  58.8  &   58.8 &   58.8      \\ \hline
70\%       &58.8                       & 70.5   &  {\bf 76.4 }  & 64.7   &  64.7  &   64.7 &  70.5  &  76.4  &    52.9&    64.7     \\ \hline
80\%       &58.8                       & 70.5   &  70.5  &   58.8  &  {\bf 76.4}   &  64.7  & 76.4   &  70.5  &   58.8 &    64.7     \\ \hline
90\%      &58.8                        & 70.5   &  70.5   &  58.8   & {\bf 76.4 }  &  76.4  &   70.5 &  76.4  &  64.7  &    64.7    \\ \hline
100\%    &70.5                      &  64.7  & 70.5    &   64.7 &  70.5  &    76.4  &  {\bf 82.3} & 82.3   &   70.5 &     64.7    \\ \hline
\end{tabular}
\caption{\footnotesize Classification accuracy for varying number of features and instances (Embryo) }
\label{table:fs_is_evaluation_embro}%\vsa\vsa
\end{table}
